# Supplementary material for: Topology of Wilson-loop spectrum and periodic evolution of surface-state Fermi arc
Source: arXiv:2303.10178 source file (2023-03-17)
Supplement: Supplementary file 1 [file Supplementary.pdf]

# Supplementary Material

## S1. ESTABLISHING TOPOLOGICAL EQUIVALENCE BETWEEN WILSON-LOOP SPECTRUM AND "BOUNDARY FERMI SURFACE"

The boundary-state spectrum is shown to be the deformation of the Wilson-loop spectrum in ref.[1]. Here we use a simplified version of the model used in ref.[1] to prove the topological equivalence between Wilson-loop spectrum and "boundary Fermi surface". We use the hybrid Wannier representation to build the model for the boundary. $|\Psi^j_{R_x,\mathbf{k}_{||}}\rangle$ denotes the Wannier function around lattice $R_x$ in the $x$-direction. $\mathbf{k}_{||}$ is wave vector in the direction that parallels to the boundary. $j = 1, ...N_{occ}$ and $N_{occ}$ is the number of the occupied bands. $|\Psi^j_{R_x,\mathbf{k}_{||}}\rangle$ is an eigenfunction of $P_{\mathbf{k}_{||}} X P_{\mathbf{k}_{||}}$, where $P_{\mathbf{k}_{||}}$ projector to the occupied space for a given $\mathbf{k}_{||}$ and $X$ is the $x$-direction position operator. The eigenvalues of $P_{\mathbf{k}_{||}} X P_{\mathbf{k}_{||}}$ are the Wannier centers $\nu^j_{R_x,\mathbf{k}_{||}}$. The Wilson-loop along $x$-direction has eigenvalues $e^{i2\pi\nu^j_{R_x,\mathbf{k}_{||}}}$. We refer $\nu^j_{R_x,\mathbf{k}_{||}}$ to Wilson-loop spectrum.

The projection operator the occupied bands can be expressed as $P = \sum_{\mathbf{k}_{||},R_x,j} |\Psi^j_{R_x,\mathbf{k}_{||}}\rangle\langle\Psi^j_{R_x,\mathbf{k}_{||}}|$. We also use the spectrally flat tight-binding Hamiltonian $H = 1 - 2P$ for the system. We choose the Hamiltonian for boundary as

$$H_e = \sum_{\mathbf{k}_{||},R_x,j} V(\nu^j_{R_x,\mathbf{k}_{||}})|\Psi^j_{R_x,\mathbf{k}_{||}}\rangle\langle\Psi^j_{R_x,\mathbf{k}_{||}}| + 1 - P. \quad \text{(S1)}$$

$V(x)$ continuously connects 1 and $-1$ in an interval $x \in [-a, a]$, where $2a$ is the width of the boundary. For simplicity, we assume $V(x)$ is a continuous monotonically decreasing function of $x$. The first term in $H_e$ approaches $-P(P)$ when $\nu^j_{R_x,\mathbf{k}_{||}} > a(\nu^j_{R_x,\mathbf{k}_{||}} < -a)$ because the Wannier function is localized. So $H_e$ approaches $H$ to the right and approaches 1 to the left. Thus $H_e$ models the boundary between $H$ and vacuum. It is clear that the Wannier functions of the occupied bands are eigenfunctions of $H_e$ with eigenvalues that depend only on $\nu^j_{R_x,\mathbf{k}_{||}}$. The Wannier functions with $-a \le \nu^j_{R_x,\mathbf{k}_{||}} \le a$ correspond to boundary states. So the boundary spectrum $V(\nu^j_{R_x,\mathbf{k}_{||}})$ is a continuous deformation of Wilson-loop spectrum $\nu^j_{R_x,\mathbf{k}_{||}}$. For example when $V(x) = -x/a$, the boundary-state spectrum is just Wilson-loop spectrum $\nu^j_{R_x,\mathbf{k}_{||}}$ with a scaling. Usually the boundary-state spectrum only contains part of information of Wilson-loop spectrum. For example when $a < 1/2$ only part of the Wilson-loop spectrum (defined modulo 1) is in the boundary area $-a \le x \le a$. The rest of the Wannier functions merge to the bulk bands as is shown in Fig.S1 (c) and (d). This conclusion is generally true in the original model with open boundary condition as is shown in Fig.3 (e) and (f) and Fig.4 (c) and (d). So we can not obtain the full topological information of Wilson-loop by observing the boundary-state spectrum alone.

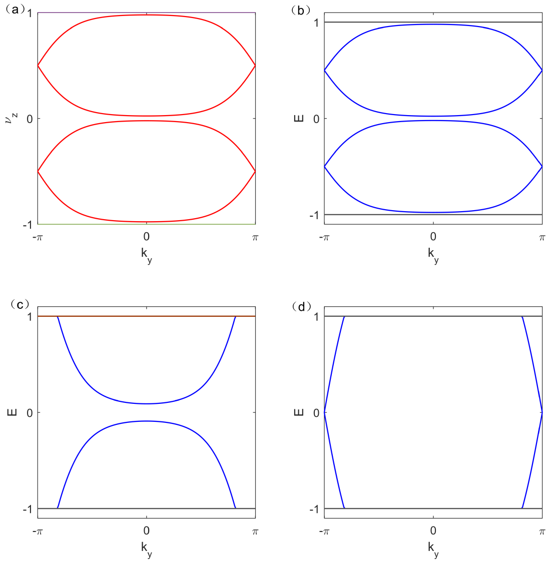


FIG. S1. (a)Wilson-loop spectrum of the 2D trivial insulator in the main text . (b)-(d) Energy spectrums of spectrally flat model of the boundary with different $a$ and $\phi_d$. $\phi_d = 0$ in (b) and (c) and $\phi_d = 0.5$ in (d). $a = 1$ in (b) and $a = 1/4$ in (c) and (d).

Now we design a continuous periodic process that one layer of unit cells of the system are removed in one period. We can keep the boundary fixed and continuously translate the system to the left in the $x$-direction. When the system is translated by one lattice constant the system will return to its original state and thus the process can be considered as periodic. In this process one layer of unit cells move out of the system. To simulate this process we can keep the system fixed and continuously move the boundary to the right.

When the boundary is moved by $\phi_d$ and $V(x)$ becomes $V(x-\phi_d)$ and the eigenenergy becomes $V(\nu^j_{\mathbf{k}_{||}i} - \phi_d)$. We assume the Fermi level $E_f$ is at the bulk gap, that is $-1 < E_f < 1$, and $V(x) = E_f$ has a single solution $\nu_0$. Then the Fermi arc for a given $\phi_d$ is determined by $\nu^j_{R_x,\mathbf{k}_{||}} - \phi_d = \nu_0$. For a given $\mathbf{k}_{||}$ the $\phi_d$s that make the surface state at the Fermi level satisfies $\phi_d(\mathbf{k}_{||}) = \nu^j_{R_x,\mathbf{k}_{||}} - \nu_0$, which shows that $\phi_d(\mathbf{k}_{||})$ and $\nu^j_{R_x,\mathbf{k}_{||}}$ are congruent. In this way we show the topological equivalence between the surface generated by evolution of Fermi arc and the Wilson-loop spectrum. The solution of $\nu^j_{R_x,\mathbf{k}_{||}} - \phi_d = \nu_0$ exist for every $\mathbf{k}_{||}$, so the Fermi arc will sweep the whole boundary Brillouin zone.

## S2. FROM THE SPECTRALLY FLAT HAMILTONIAN TO THE ORIGINAL HAMILTONIAN

Now we discuss whether the results obtained by using spectrally flat Hamiltonian are still correct when the original tight-binding model is used. The spectrally flat Hamiltonian can be continuously connected to the original model with a boundary by gradually turning on the hopping terms between the Wannier functions and continuously changing the average energy of the Wannier functions. Some of the Wannier functions near the boundary continuously evolve to boundary states and the others evolves to the bulk states. Part of the Wilson-loop spectrum evolves to the boundary-state spectrum. The bulk gap does not close in this process.

The first question is whether the boundary-state spectrum of the original model is still the partial deformation of the Wilson-loop spectrum. It is claimed that the topology of the boundary-state spectrum will not change under continuous deformation in ref.1. However, there are systems with symmetry-protected gapless Wilson-loop spectrum but gapped boundary-state spectrum,e.g. the inversion-symmetric TI[2]. So we need to show under what condition does the partial topological equivalence between Wilson-loop spectrum and boundary-state spectrum in original model exist.

The gaplessness of the Wilson-loop spectrum depends on the symmetry protected degeneracies at the special $\mathbf{k}_{||}$s. For example, in 2D TIs the Wilson-loop spectrum is degenerate at $k_{||} = 0, \pi$ due to the time-reversal symmetry. These degeneracies are bulk property because they are independent of the boundary of the system. However, when boundary presents, the symmetry of the bulk system may be broken. For example, the presence a boundary bounds to break the inversion symmetry of the inversion-symmetric TI. In this case the spectrally flat model may exhibit a gapless boundary-state spectrum. However, the boundary-state spectrum of original tight-binding model becomes gapped as is shown in Fig.S2 b due to the presence of the boundary.

In comparison the Kramer degeneracy of the boundary states still exist as long as the boundary of the original system preserve the time-reversal symmetry. So boundary states in 2D and 3D TIs are gapless while the boundary states of inversion-symmetric TIs are gapped in general.

Another example is shown in Fig.3 (c)-(f). This system is trivial because the Wilson-loop spectrum is gapped. However, the gapless edge state spectrum can be observed because the degeneracy of Wilson-loop spectrum at $k_y = \pi$. Though this model break the time-reversal symmetry, the symmetry-breaking term disappears at the $k_y = \pi$. So this degeneracy is not broken by the presence of the boundary when $k_y$ can still be defined. That is, this degeneracy is still protected by the time-reversal symmetry. In conclusion, the boundary-state spectrum is a partial deformation of Wilson-loop spectrum when

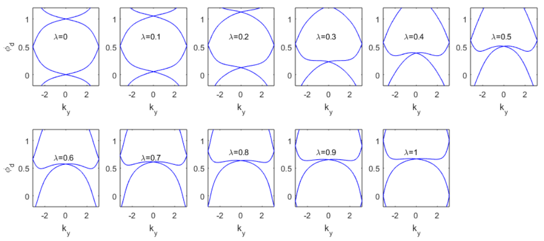


FIG. S2. Evolution of "boundary Fermi arc" with $\lambda$.The model for 2D TI discussed in the main text is used here. $U_0 = 1000$ is used to approximate $U_0 = +\infty$ in the simulation. Fermi energy is chosen to be $E_f = 0$.

the symmetry-protected degeneracy is not split by the presence of boundary.

The next question is whether the "boundary Fermi surface" is still topologically equivalent to the Wilson-loop spectrum when the original tight-binding model is used. The answer is that they are topologically equivalent when the symmetry-protected degeneracy of Wilson-loop spectrum is not split when it evolves to the boundary-state spectrum of the original model.

The spectrally flat Hamiltonian for the boundary can be continuously connected to the original Hamiltonian with a boundary while keeping the bulk gap open. So the process discussed in the S1 can be continuously deformed to a process with original model. Now the question becomes whether the topology of "boundary Fermi surface" will remain unchanged in this deformation. There are two possible topological changes the "boundary Fermi surface" may experience in the deformation: the accidental degeneracy of the "boundary Fermi surface" may be split and new accidental degeneracy maybe created. Since the accidental degeneracy does not affect the topology of Wilson-loop spectrum[3], the "boundary Fermi surface" of the original model still preserve the topological information of the Wilson-loop spectrum.

In comparison the degeneracies of Wilson-loop spectrum that are protected by the inversion symmetry will be split by the presence of a boundary. Thus the "boundary Fermi surface" of the inversion symmetric TI is gapped while the Wilson-loop spectrum is gapless as is shown in Fig. S2 a and c.

To illustrate the continuous deformation from the spectrally flat model to the original model we consider a model with a continuous parameter $\lambda$. The Hamiltonian $H_\lambda(\phi_d) = (1-\lambda)H_e(\phi_d) + \lambda H_0(\phi_d)$ continuously varies from the spectrally flat Hamiltonian to the original Hamiltonian when $\lambda$ continuously varies from 0 to 1, where $H_e(\phi_d)$ is the spectrally flat Hamiltonian for boundary with given $\phi_d$ and $H_0(\phi_d)$ is the Hamiltonian for the original model with a boundary. The boundary is created by adding onsite potential $U(R_x - \phi_d)$ to the bulk model. $U(x)$ is a continuous decreasing function and it approaches to 0 in the system.

In most of the researches the open boundary condition

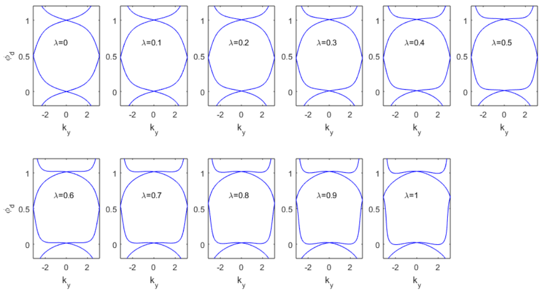


FIG. S3. Evolution of "boundary Fermi arc" with a different $U(x)$. The same model in Fig.S2 is used. $U(x) = 2(1 - \tanh(4x))$ is used. Fermi energy is chosen to be $E_f = 0$.

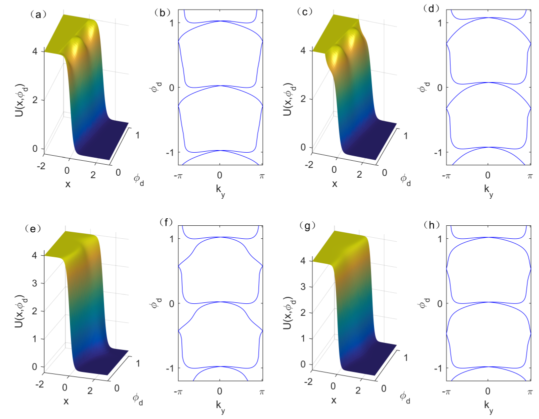


FIG. S4. The "boundary Fermi surface" with a $\phi_d$-dependent $U(x, \phi_d)$. (a) and (b),$U(x, \phi_d) = 0.2\sin^2(2\pi\phi_d)U_1(x - \phi_d) + (1 - 0.2\sin^2(2\pi\phi_d))U_2(x - \phi_d)$, where $U_1(x)$ is the potential used for open boundary condition with $U_0 = 4$ and $U_2(x) = 2(1 - \tanh(4x))$. In (a) we show $U(x, \phi_d)$ is not just a translation of the same $U(x)$. The form of $U(x, \phi_d)$ also varies with $\phi_d$. (b) The "boundary Fermi surface" when the boundary potential is $U(R_x, \phi_d)$. (c)-(h),Other three types of $\phi_d$-dependent $U(x, \phi_d)$ are used. $U(x, \phi_d) = 0.2\cos^2(2\pi\phi_d)U_1(x - \phi_d) + (1 - 0.2\cos^2(2\pi\phi_d))U_2(x - \phi_d)$ in (c) and (d), $U(x, \phi_d) = 2(1 - \tanh(4(1 + \sin(2\pi\phi_d)(x - \phi_d))$ in (e) and (f) and $U(x, \phi_d) = 2(1 - \tanh(4(1 + \cos(2\pi\phi_d)(x - \phi_d))$ in (g) and (h).

is used. The open boundary in our work is realized by by using $U(x) = (1-x)/(x+1/U_0)$ when $0 \leq x \leq 1$. $U(x) = 0$ inside the system($x \geq 1$) and $U(x) = U_0$ outside of the system ($x \leq 0$). The open boundary is achieved by letting $U_0 \to +\infty$. When $\phi_d = 0(\phi_d = 1)$ $U(R_x - \phi_d) = +\infty$ if $R_x \leq 0$ ($R_x \leq 1$) and $U(R_x - \phi_d) = 0$ if $R_x \geq 1$ ($R_x \geq 2$). This is just the open boundary condition used in most of the researches. So the periodic process can be realized by changing the onsite potential of the layer of unit cells with $R_x = 1$. That is, we continuously remove one layer of unit cells from the system by continuously increasing the onsite potential of this layer of unit cells. All the results in main text are obtained by using this type of $U(x)$ for open boundary conditions.

Here we use two different types of $U(x)$ to show the "boundary Fermi surfaces" are continuous deformations of Wilson-loop spectrums in Fig. S2 and S3. The results show the "boundary Fermi surface" is strictly equivalent to the Wilson-loop spectrum. To show the topology of "boundary Fermi surface" does not depends on the specific $U(x)$ we also change the form of $U(x)$ when $\phi_d$ changes as is shown in Fig.S4. All these results shows the "boundary Fermi surface" can be observed when one layer of unit cells is continuously removed from the system and the observing process does not depends on the specific way of removing the unit cells.

[1] L. Fidkowski, T. S. Jackson, and I. Klich, Phys. Rev. Lett. **107**, 036601 (2011).

[2] A. Alexandradinata, X. Dai, and B. A. Bernevig, Phys. Rev. B **89**, 155114 (2014).

[3] R. Yu, X. L. Qi, A. Bernevig, Z. Fang, and X. Dai, Phys. Rev. B **84**, 075119 (2011).
